# Supplementary material for: Revisiting Perspective Information for Efficient Crowd Counting
Source: arXiv:1807.01989 source file (2019-04-01)
Supplement: Supplementary file 1 [file sec-appendix.tex]

\appendix \label{Sec:Perspective}
%\holger{Headline should just be appendix and perspective estimation a section below that.}
%This appendix details the computation of $\frac{{\partial {L_{{\mathrm D}}}}}{{\partial {\alpha}}}$ and $\frac{{\partial {L_{{\mathrm D}}}}}{{\partial {\beta}}}$ ($t$ is omitted for simplicity) in (\ref{Eq:paraupdate}). Recalling the notations in (\ref{Eq:DensityWeight})(\ref{Eq:Weight}) and Sec.~\ref{Sec:Architecture}, we write out the chain rule:
%\begin{equation}\label{Eqn: diffalpha}
%\begin{aligned}
%\frac{{\partial {L}}}{{\partial \alpha }} &= \frac{{\partial L}}{{\partial {D^e}}}\frac{{\partial {D^e}}}{{\partial W}}\frac{{\partial W}}{{\partial \alpha }}\\
% &= \frac{{\partial L}}{{\partial {D^e}}}({D^{{e_1}}} - {D^{{e_2}}})\frac{{\partial W}}{{\partial \alpha }}\\
% &= \frac{{\partial L}}{{\partial {D^e}}}\sum\nolimits_j {(d_j^{{e_1}} - d_j^{{e_2}})} \frac{{\partial {w_j}}}{{\partial \alpha }}\\
% &= \frac{{\partial L}}{{\partial {D^e}}}\sum\nolimits_j {(d_j^{{e_1}} - d_j^{{e_2}})(p_j^e - \beta )f(p_j^e)(1 - f(p_j^e))}
%\end{aligned}
%\end{equation}
%Similarly, we have
%\begin{equation}\label{Eqn: diffbeta}
%\begin{aligned}
%\frac{{\partial {L}}}{{\partial \beta }} = \frac{{\partial L}}{{\partial {D^e}}} \sum\nolimits_j (d_j^{{e_1}} - d_j^{{e_2}})( - \alpha )f(p_j^e)(1 - f(p_j^e))
%\end{aligned}
%\end{equation}
\emph{This supplementary material provides the experimental results for perspective estimations. We evaluate perspective estimations on ShanghaiTech dataset~\cite{zhang2016cvpr} following the same implementation details as in Sec.4.2. We first present the evaluation protocol and then offer the results.}

\medskip

\para{Evaluation Protocol.} The final perspective maps produced by PACNN are of $\frac{1}{8}$ resolution of the ground truth maps. To compare with the ground truth, we downsample the ground truth maps to have the same resolution. We normalize both the estimated and ground truth perspective values within each map for comparison.

%(${p_j} \leftarrow  \frac{{{p_j} - {{\min }_p}}}{{{{\max }_p} - {{\min }_p}}}$).

For each estimated perspective map $P^e$, we employ three measurements to evaluate its similarity to the ground truth $P^g$:
mean absolute perspective error (MAE$_\text P$), root mean squared perspective error (RMSE$_\text P$), and peak perspective signal to noise ratio (PSNR$_\text P$),
\begin{equation}\label{Eq:MAE}
\begin{split}
&\mathrm{MAE_P} = \frac{1}{{S}}\sum\limits_{j = 1}^S {|{{p^e_j} - {p^g_j}}|},\\
&\mathrm{RMSE_P} = \sqrt{\frac{1}{{S}}\sum\limits_{j = 1}^S {({{p^e_j} - {p^g_j}})^2}},\\
&\mathrm{PSNR_P} = 20 \log_{10} (\frac{\mathrm{MAX_P}}{\mathrm{RMSE_P}})
\end{split}
\end{equation}
where $p^e_j$ and $p^g_j$ denote the normalized estimated and ground truth perspective values at pixel $j$, respectively. We use $S$ to denote the total number of pixels in each map. $\mathrm{MAX_P}$ is the maximum possible pixel value of the perspective map $P$. Since both $P^e$ and $P^g$ are normalized,
$\mathrm{MAX_P} = 1$ in practice. We average the MAE$_\text P$, RMSE$_\text P$ and PSNR$_\text P$ over the entire set, and denote by $\overline {\mathrm{MAE_P}}$, $\overline {\mathrm{RMSE_P}}$ and $\overline {\mathrm{PSNR_P}}$ our final measurements. Small $\overline {\mathrm{MAE_P}}$ and $\overline {\mathrm{RMSE_P}}$ and big $\overline {\mathrm{PSNR_P}}$ indicate good performance.
\medskip

%\begin{table}[t]
%	\setlength{\tabcolsep}{2.6pt}
%	\centering
%	\small
%	\begin{tabular}{|c||c|c|c|}
%		\hline
%	 Examples in Fig.~\ref{Fig:PMAP} &  $ {\mathrm{MAE_P}}$ & ${\mathrm{RRMSE_P}}$ & $ {\mathrm{PSNR_P}}$ \\
%		\hline
%		top-left& 0.093& 0.129 & 17.80\\
%		top-right & 0.075 & 0.089 & 20.50 \\
%		bottom-left& 0.090 & 0.121 & 18.31\\
%		bottom-right & 0.126  & 0.152 & 16.40 \\
%		\hline
%	\end{tabular}
%	%   \pretabspace
%	\caption{Evaluations of Examples in Fig.~\ref{Fig:PMAP}. ${\mathrm{MAE_P}}$, ${\mathrm{RRMSE_P}}$ and $ {\mathrm{PSNR_P}}$ are reported.}
%	\label{Tab:Example}
%	%   \posttabspace
%\end{table}

\para{Results on ShanghaiTech.} We show the perspective map estimation results in Table~\ref{Tab:Perspective} on ShanghaiTech PartA and PartB, respectively. $\overline {\mathrm{MAE_P}}$, $\overline {\mathrm{RMSE_P}}$ and $\overline {\mathrm{PSNR_P}}$ are similar between PartA and PartB. Their $\overline {\mathrm{PSNR_P}}$ are 18.98, and 17.94, respectively. We illustrated some examples in Fig.3 in the paper: 
%; Top left: 0.093 (MAE$_\text P$), 0.129 (RRRMSE$_\text P$), 17.80 (PSNR$_\text P$); Top right: 0.075, 0.089, 20.5; Bottom left: 0.090, 0.121, 18.31; Bottom right: 0.126, 0.152, 16.4.  
the estimated perspective map in general reflects the perspective distortion as in the corresponding ground truth, albeit the noise. 
%In Table.~\ref{Tab:Shanghaitech} we show the crowd counting accuracy using the estimated perspective maps is in fact very close to that using the ground truth perspective maps.
%\holger{Only use the word precision if you mean the same as in precision and recall.}

\begin{table}[t]
	\setlength{\tabcolsep}{2.6pt}
	\centering
	\small
	\begin{tabular}{|c|c|c|c|}
		\hline
		ShanghaiTech &  $\overline {\mathrm{MAE_P}}$ & $\overline {\mathrm{RMSE_P}}$ & $\overline {\mathrm{PSNR_P}}$ \\
		\hline
		PartA& 0.089 & 0.112 & 18.98\\
		PartB & 0.111  &  0.134 & 17.94 \\
		\hline
	\end{tabular}
	%   \pretabspace
	\caption{Perspective estimations using PACNN. $\overline {\mathrm{MAE_P}}$, $\overline {\mathrm{RMSE_P}}$ and $\overline {\mathrm{PSNR_P}}$ are the mean values of MAE$_\text P$, RMSE$_\text P$, and PSNR$_\text P$ over the dataset.}
	\label{Tab:Perspective}
	%   \posttabspace
\end{table}
